# Supplementary material for: Mirror Symmetry for Quiver Algebroid Stacks
Source: arXiv:2206.03028 source file (2025-09-30)
Supplement: Supplementary file 1 [file Relations_of_quiver_algebra.pdf]

# Relations of quiver algebra

Monday, November 1, 2021

1:10 PM

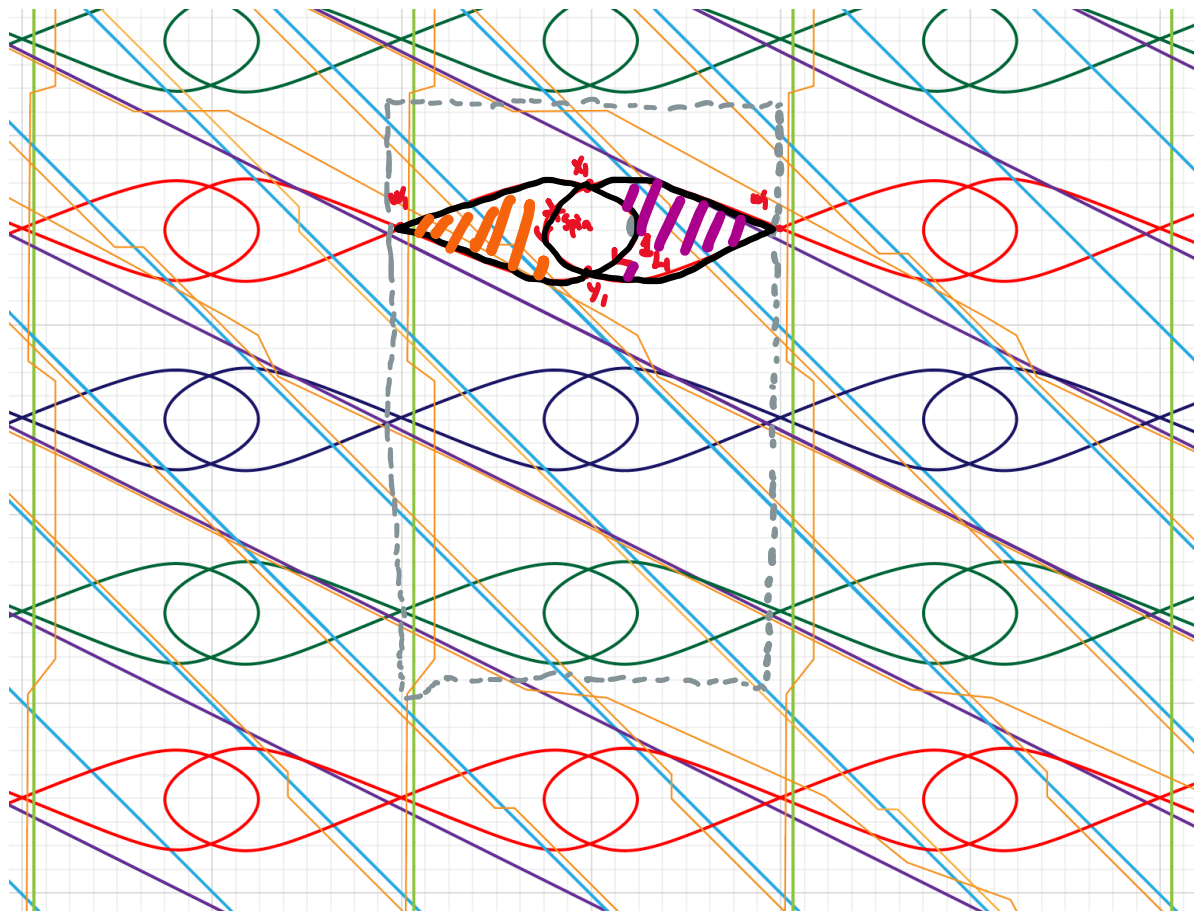

Area of shaded region is  $A_3 + A'_1 - A'_2 - A'_4$

Area of unshaded region is  $A'_3 + A_1 - A_2 - A_4$

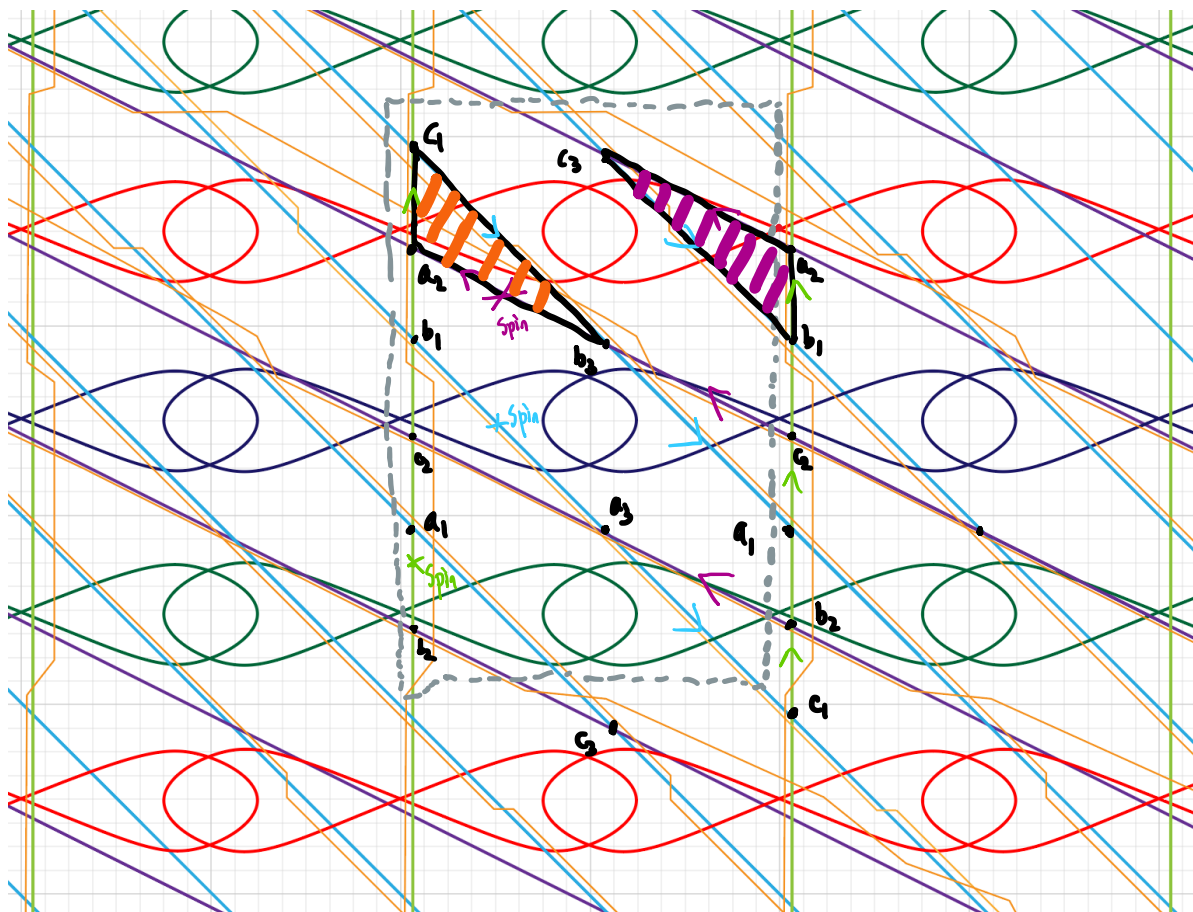

$T^{A'}_{c_1 b_3} - T^{A_1}_{b_1 c_3}$

Area of orange triangle =  $A'_1$   
 ...purple triangle =  $A_1$
